# Supplementary material for: Private Data Valuation and Fair Payment in Data Marketplaces
Source: arXiv:2210.08723 source file (2023-02-17)
Supplement: Supplementary file 1 [file Appendix.tex]

\section{Appendix}

\subsection{Details of Datasets Used in Section~\ref{sec:experiments_for_utility}}
\label{ssec: datasets}
(1) \textsl{a9a}~\footnote{\url{https://www.csie.ntu.edu.tw/~cjlin/libsvmtools/datasets/binary.html\#a9a}}~\cite{zeng2008fast} is a classical census dataset for training a model to predict whether a person makes over \$50K a year. It has \numprint{48842} samples in total including \numprint{32561} training samples and \numprint{16281} testing samples. Each sample has 124 features. We used it as benchmark for tabular dataset. 

(2) \textsl{MNIST}~\cite{lecun-mnisthandwrittendigit-2010} is one of the most popular dataset in ML, and has been widely used in Image-recognition. It has \numprint{60000} training samples and \numprint{10000} testing samples. The images are 28×28 gray scale pixels. 

(3) \textsl{USPS}~\cite{Dua:2019} is also a handwritten digits dataset of \numprint{9298} images. The images are 16×16 gray scale pixels. 

(4) \textsl{CIFAR-10}~\cite{krizhevsky2009learning} consists of \numprint{60000} 3-channel images in 10 classes. Each image is of size 32 × 32. 

(5) \textsl{STL-10}~\cite{coates2011analysis} is inspired by the CIFAR-10 dataset but with some modifications. It has 500 training images (10 pre-defined folds) and 800 test images per class. The images are 96×96 color scale pixels. 

%====================================================================

\subsection{Structure of the data utility model}
\begin{table}[htb]
\begin{tabularx}{8.6cm}{c|l}  
\toprule 
\multirow{2}{*}{$G_f$} & \makecell[l]{Convolution: input image $28 \times 28$, window size \\$4 \times 4$, stride (2, 2), number of output channels of \\16: $\mathbb{R}^{16\times14\times14}\leftarrow \mathbb{R}^{1\times28\times28}$} \\\cline{2-2}
& Square Activation\\
\midrule 
\multirow{4}{*}{$f_{DS}$} & \makecell[l]{Fully Connected: incoming nodes 3136, outgoing \\notes: 512: $\mathbb{R}^{512}\leftarrow \mathbb{R}^{3136}$} \\\cline{2-2}
& Average Operation\\\cline{2-2}
& \makecell[l]{Fully Connected: incoming nodes 512, outgoing\\ notes 256: $\mathbb{R}^{256}\leftarrow \mathbb{R}^{512}$} \\\cline{2-2}
& \makecell[l]{Fully Connected: incoming nodes 256, outgoing \\notes 1: $\mathbb{R}\leftarrow \mathbb{R}^{256}$} \\
\midrule 
\multicolumn{2}{l}{Sigmoid Activation}
\midrule  
\bottomrule 
\end{tabularx} 
\caption{The structure of the data utility function for MNIST.}
\label{tab:utility_funcition_mnist}
\end{table}

\begin{table}[htb]
\begin{tabularx}{8.6cm}{c|l}  
\toprule 
\multirow{4}{*}{$G_f$} & \makecell[l]{Convolution: input image 3 × 32 × 32, window \\size 5 × 5, stride (2, 2), number of output \\channels of 16: $\mathbb{R}^{16\times16\times16}\leftarrow \mathbb{R}^{3\times32\times32}$} \\\cline{2-2}
& Square Activation\\\cline{2-2}
& \makecell[l]{Convolution: window size 5 × 5, stride (2, 2),\\ number of output channels of 32:\\ $\mathbb{R}^{32\times8\times8}\leftarrow \mathbb{R}^{16\times16\times16}$} \\\cline{2-2}
& Square Activation\\
\midrule 
\multirow{4}{*}{$f_{DS}$} & \makecell[l]{Fully Connected: incoming nodes 2048, outgoing \\notes: 512: $\mathbb{R}^{512}\leftarrow \mathbb{R}^{2048}$} \\\cline{2-2}
& Average Operation\\\cline{2-2}
& \makecell[l]{Fully Connected: incoming nodes 512, outgoing\\ notes 256: $\mathbb{R}^{256}\leftarrow \mathbb{R}^{512}$} \\\cline{2-2}
& \makecell[l]{Fully Connected: incoming nodes 256, outgoing \\notes 1: $\mathbb{R}\leftarrow \mathbb{R}^{256}$} \\
\midrule 
\multicolumn{2}{l}{Sigmoid Activation}

\midrule  
\bottomrule 
\end{tabularx}   
\caption{The structure of the data utility function for CIFAR-10.}
\label{tab:utility_funcition_cifar10}
\end{table}
